# Supplementary material for: Spurious Feature Eraser: Stabilizing Test-Time Adaptation for Vision-Language Foundation Model
Source: arXiv:2403.00376 source file (2025-01-14)
Supplement: Supplementary file 1 [file appendix.tex]

\appendix
\onecolumn

\tableofcontents

\section{Details of Construction of Auxiliary Images}\label{sec:app-sam}

\subsection{SAM Family}
In addition to the language foundation model and visual-text foundation model, numerous of foundation models for image segmentation have recently been released. $\bullet$ Segment anything (SAM)~\cite{kirillov2023segment} released by Meta AI Research effectively segments images into foreground and background, enabling us to approximate the differentiation between spurious features and task-relevant features. Besides the general-purpose segmentation foundation models, there has been significant progress in task-specific segmentation models. For instance, $\bullet$ MedSAM~\cite{ma2023segment} specializes in medical image segmentation, while $\bullet$ Track anything (TAM)~\cite{yang2023track} focuses on object tracking and segmentation in the field of video. As segmentation models continue to advance in various domains, the applicability and flexibility of our proposed method will also enhance. $\bullet$ SAM-Med3D~\cite{wang2023sammed} introduce a foundation model for segmenting 3D medical images, such as CT and MRI sequences.

\subsection{Construct Auxiliary Images with SAM}
As a segmentation foundation model, SAM can effectively segment the content of any image based on prompts, such as ``{\tt the [object(s)] in the image}" In this work, we do not assume prior knowledge of the actual objects in the image. Therefore, for benchmark datasets like PACS and Waterbirds, we use an empty string as the segmentation prompt. On the other hand, for datasets constructed through \ste, we use a generic term encompassing all categories to ensure accurate segmentation (i.e., we use ``the animals in the image" as the segmentation prompt for animal classification tasks).

\begin{figure}[th]
    \centering
    \includegraphics[width=0.68\linewidth]{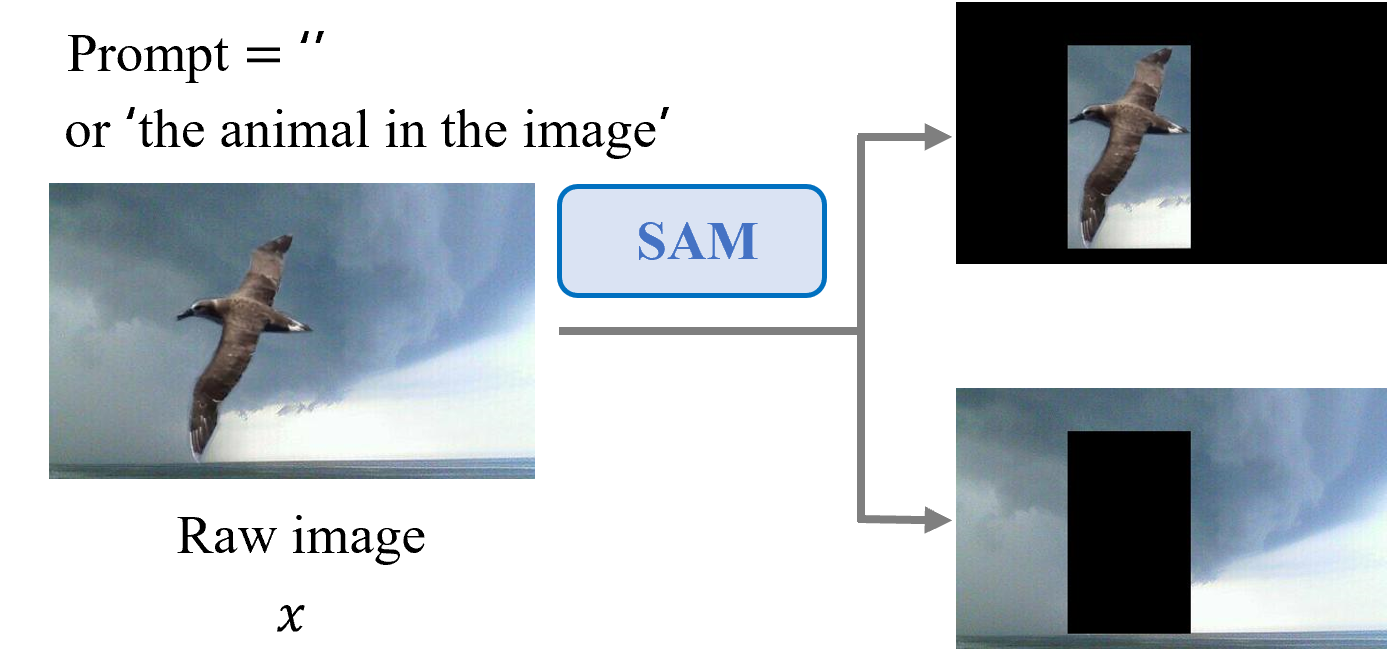}

        \caption{Illustration of the usage of SAM.}
    \label{fig:sam}
\end{figure}

It is worth mentioning that even when using a completely empty string as a prompt for foreground segmentation, SAM is still able to accurately segment the scene to a large extent, except for some relatively complex backgrounds.

\section{Some Decision Shortcuts are Not Severe in BLIP-2}\label{sec:app_blip}
\subsection{Observations}
As shown in the main text, on the Waterbirds dataset, the model exhibits clear decision shortcuts, specifically in the form of poor performance on the worst group. We believe that when a model predicts incorrectly on raw images but correctly on the foreground, it indicates the presence of a decision shortcut on the background of that sample. However, we do not observe any significant background shortcuts in the CamelDeer dataset (only a 2\% improvement is achieved after masking out the background.). In other words, BLIP2 is able to perform relatively accurate classification on raw images for this dataset.
\subsection{Analyses}
\begin{table}[ht]
  \centering
  \caption{Zero-shot classification performance of BLIP-2. }\label{tab:blip_other}
{
  % \resizebox{\columnwidth}{!}{
    \begin{tabular}{cc|ccc}
    \toprule
    {Dataset}& & {Vanilla} & {Ours}\\
    \midrule 

\multirow{2}{*}{CamelDeer}&$\text{AVG.}$ &$98.2$ &$99.0$\\
&$\text{W.G.}$  &$97.2$   &$98.4$ \\
    \midrule 

\multirow{2}{*}{SpiderCrab}&$\text{AVG.}$ &$88.2$ &$97.4$\\
&$\text{W.G.}$  &$82.8$  &$95.6$ \\

    \bottomrule
    \end{tabular}}%
\end{table}

As shown in the Table.~\ref{tab:blip_other}, the performance of BLIP-2 has been improved after applying \eraser, which proves that the objects in the images are discernible, and the misclassifications by the CLIP model are due to decision shortcuts caused by the background.

\section{More Design Choices}
\subsection{Patches Shuffle}
We attempt to deploy a method when there is no SAM annotation at all, meaning no tools are used to distinguish foreground and background. We simulate 
auxiliary images using the method shown in the figure below. Specifically, we randomly disrupt the information in the image by scrambling the entire image into patches of size 4 as auxiliary images.

\begin{figure}[ht]
    \centering
    \includegraphics[width=0.55\linewidth]{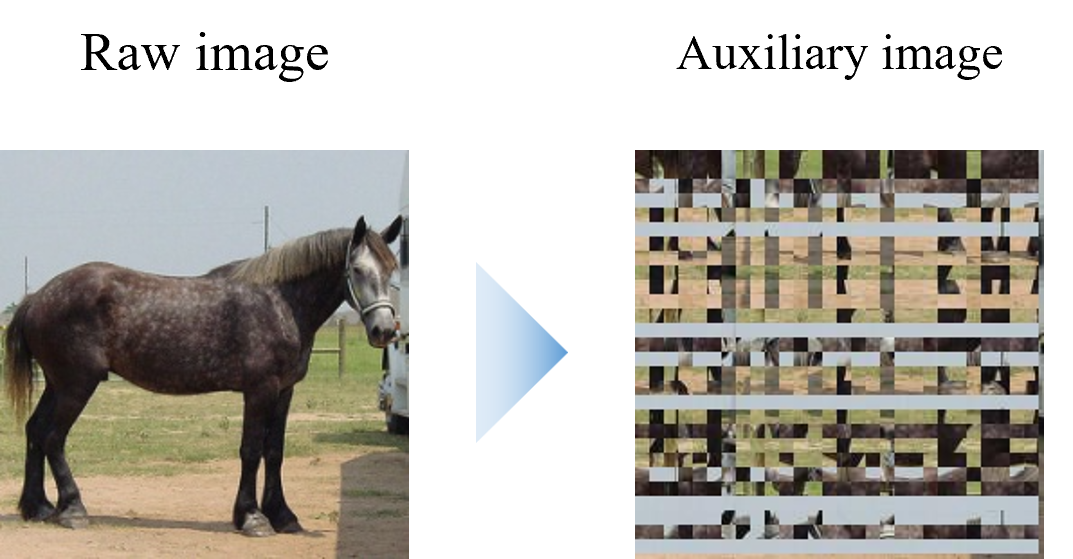}

        \caption{Illustration for shuffling patches.}
    \label{fig:wosam}
\end{figure}

The proposed method still be deployed when there is absolutely no task-relevant annotation information available.

\subsection{Empirical Results}
We test the performance of our proposed method in extreme scenarios where no spurious features annotation information could be obtained. We directly replace the foreground marked in SAM with the entire original image and randomly shuffled the background marked in SAM using pixel values, as shown in Fig.~\ref{fig:wosam}.

\begin{table}[ht]
  \centering
  \caption{Zero-shot accuracy performance for Vanilla CLIP and SEraser, where ``w/o Anno.'' indicates the absence of an annotation model like SAM, and the task-irrelevant features are simulated as shown in Fig.~\ref{fig:wosam}.}\label{tab:wosam}
{
  % \resizebox{\columnwidth}{!}{
    \begin{tabular}{cc|cc}
    \toprule
    \multicolumn{2}{c}{Dataset} & {Vanilla}& Ours (w/o Anno.)\\
    \midrule 
    \multirow{2}{*}{Waterbirds}
    &$\text{AVG.}$ &$67.67$ &$72.30_{0.20}$  \\
    &$\text{W.G.}$  &$40.04$ &$48.78_{0.56}$\\
    \midrule 
     \multirow{2}{*}{CamelDeer}
    &$\text{AVG.}$ &$83.20$ &$83.73_{0.09}$ \\
    &$\text{W.G.}$ &$66.40$ &$67.47_{0.19}$ \\ %gap $16.27_{0.09}$
    \midrule 
    \multirow{2}{*}{SpiderCrab}
    &$\text{AVG.}$ &$66.00$ &$77.33_{0.38}$ \\
    &$\text{W.G.}$ &$42.00$ &$64.27_{0.68}$ \\
    \midrule 
  \multirow{2}{*}{PACS} & $\text{AVG.}$ &$91.75$  &$92.21_{0.00}$\\
&$\text{W.G.}$  &$59.08$  &$67.68_{0.11}$ \\
    %gap $13.07_{0.50}$

    \bottomrule
    \end{tabular}}%
\end{table}

As shown in Table~\ref{tab:wosam}, even when using randomly perturbed images as spurious features in \eraser, it can still improve (at least without decreasing) CLIP zero-shot classification performance. In other words, our method can still be deployed even without any information that can separate spurious and task-relevant features. The strategy shown in Fig.~\ref{fig:wosam} is just a simple alternative, and in practical applications, we may have more proxy spurious features. For example, in intelligent healthcare and medical image recognition, the lesions annotated by doctors can be considered as task-relevant features, while other locations can be regarded as spurious features. A high-quality annotation agent can guarantee better performance for our method. However, the paradigm proposed in this paper does not strictly depend on any specific annotation agent.

\section{Supplements of Related Work}
Apart from Alpha-CLIP~\cite{sun2023alpha}, there are several other recently proposed region-aware CLIP methods that require additional training sets for fine-tuning. SAM-CLIP~\cite{wang2023sam} achieves region-aware by jointly training a segment model and CLIP. Another approach is a two-stage strategy~\cite{liang2023open}, where a segmentation model is trained, followed by CLIP adaptation using collected mask-category pairs. Both of these strategies require additional training sets to train CLIP, which not only increases the chances of building new decision shortcuts on the distribution of the new training set but also incurs high retraining costs and disrupts the original weights of CLIP. The method proposed in this paper does not require additional training sets and does not disrupt the weights and architecture of CLIP. It only requires adaptation on a single test sample to a great extent eliminate decision shortcuts.

\section{Details of Datasets and Compared Methods}\label{sec:app_compared}

\subsection{Datasets and Platform}\label{sec:app-datasets}
In this paper, we compare several recently proposed methods on the platform with 8xA100 GPUs, including region-aware-clip and prompt-tuning on different datasets. As previously mentioned, VLFMs have been thoroughly trained on a large amount of data, and many decision shortcuts do not exist in these pre-trained models (at least not prominently enough to be reflected in the accuracy differences). Therefore, in this paper, we propose a new evaluation paradigm, SE. In real-world datasets, we select the five classes that perform worst on CLIP and pair them with a class that is easily confused to form a 10-class subset. This allows us to more clearly demonstrate the differences between different methods.

\subsection{Setting of Compared Methods}\label{sec:app_setting}

We compare our method with various different methods, regarding how different methods are deployed in this paper, detailed descriptions are followed.

\subsubsection{Vanilla Baseline}
As the most basic comparative method, we utilized the raw CLIP model for zero-shot classification directly, in order to observe the performance of the original model. For the prompt in this paper, we used the same prefix for all categories in each dataset, such as ``{\tt a photo of a [class]}" or ``{\tt a photo containing [class]}". We then calculated the embedding distance between the image and each text prompt to determine the closest one, which is considered as the final category. It is worth mentioning that in this paper, we scaled the softmax scores using the model's preset temperature during calculation. Specifically, the temperature value was set to 0.01.

\subsubsection{MASK Strategy}
We use SAM~\cite{kirillov2023segment} to box the foreground and mask the background, then the masked image is classified in a zero-shot classification manner, namely we didn't use any label during segmentation and just use the prompt such as ``the animal in the picture'', since we have not label during testing. When using SAM for background masking, we uniformly segment based on bounding boxes. If an image contains multiple foreground regions, we concatenate these regions to form the foreground portion.

\subsubsection{Alpha-CLIP}
which is a \emph{region-aware} version of CLIP with an auxiliary alpha channel to suggest attentive regions and fine-tuned with constructed millions of RGBA region-text pairs ~\cite{sun2023alpha}. Since this method requires an additional channel consisting of $0/1$ to mark the target region, we use the mask information to distinguish foreground and background as input for this channel. It is worth noting that this method not only adjusts CLIP on the original dataset but also constructs a large number of background mask pairs for training. Therefore, this model undergoes additional training, intuitively containing richer knowledge rather than simply adjusting based on the inherent knowledge of CLIP like other methods.

\subsubsection{Test-time Prompt Tuning}
which is a \emph{prompt tuning} method that can learn adaptive prompts on the fly with a single test sample. TPT optimizes the prompt by minimizing the entropy with confidence selection so that the model has consistent predictions across different augmented views of each test sample ~\cite{shu2022test}. This method requires view augmentation, and in our experiments, we set the number of augmentations to 32. It also requires setting a threshold for discarding samples, and we set this threshold to $\rho=0.1$ (which achieved the best performance according to the author's report).

\subsubsection{ROBOSTSHOT}
which is a method which uses zero-shot language models (LMs) to obtain useful insights from task descriptions. These insights are embedded and used to remove harmful and boost useful components in embeddings--without any supervision ~\cite{adila2023zero}. This method requires invoking a language model. In our comparative experiments, we used GPT-3.5 as the language model for this method to generate useful conceptual descriptions.

\subsection{Error Bars}\label{sec:app-errorbar}

Limited by space, the error bar are shown in Table.~\ref{tab:app-errorbar}.

\begin{table*}[ht]
  \centering
    \caption{Zero-shot classification performance for different methods with error bars.}\label{tab:app-errorbar}

{
  \resizebox{\columnwidth}{!}{
    \begin{tabular}{cc|cccccccc}
    \toprule
    \multicolumn{2}{c}{Dataset} & {Vanilla}&MASK  &{TPT} 
    & ROBOSHOT & Alpha-CLIP & {Ours}\\
    \midrule 
    \multirow{3}{*}{Waterbirds}
    &$\text{AVG.}$ &$67.67$ &$71.97$ &$66.88_{0.09}$ &$68.86$ &$67.59$ &$\pmb{78.24_{0.20}}$ \\
    &$\text{W.G.}$  &$40.04$ &$51.53$ &$34.38_{0.21}$ &$52.28$ &$43.15$ &$\pmb{65.25_{0.80}}$\\
    &$\text{GAP}$ &$27.63$ &$20.44$ &$32.50_{0.25}$ &$16.58$ &$24.44$ &${12.99_{0.61}}$\\
    \midrule 

    \multirow{3}{*}{PACS}
    &$\text{AVG.}$ &$91.75$ &$91.45$ &$92.90_{0.07}$ &$92.07$ &$\pmb{93.50}$ &$93.07_{0.05}$\\
    &$\text{W.G.}$  &$59.08$ &$60.71$ &$58.94_{0.53}$ &$66.71$ &$\pmb{73.02}$ &$68.73_{1.18}$ \\
    &$\text{GAP}$ &$32.67$ &$30.74$ &$33.97_{0.46}$ &$25.36$ &${20.48}$ &$24.34_{1.19}$ \\
    \midrule 
     \multirow{3}{*}{CamelDeer}
    &$\text{AVG.}$ &$83.20$ &$93.60$ &$77.67_{1.11}$ &$80.40$ &$92.00$ &$\pmb{95.67_{0.25}}$\\
    &$\text{W.G.}$ &$66.40$ &$87.20$ &$55.33_{2.22}$ &$60.80$ &$84.40$ &$\pmb{91.60_{0.86}}$\\
    &$\text{GAP}$ &$16.80$ &$6.40$ &$22.33_{1.11}$ &$19.60$ &$7.80$ &${4.07_{0.62}}$\\
    \midrule 
    \multirow{3}{*}{SpiderCrab}
    &$\text{AVG.}$ &$66.00$ &$91.40$ &$83.53_{0.41}$ &$73.00$ &$86.20$ &$\pmb{95.33_{0.41}}$ \\
    &$\text{W.G.}$ &$42.00$ &$90.40$ &$72.53_{0.75}$ &$50.40$ &$86.00$ &$\pmb{94.67_{1.05}}$\\
    &$\text{GAP}$ &$24.00$ &$1.00$ &$11.00_{0.49}$ &$22.60$ &${0.20}$ &$0.67_{0.66}$\\

    \bottomrule
    \end{tabular}}}%

\end{table*}

\section{Limitations}
The main limitation is the time consumption involved during deployment. Although other methods such TPT also require a considerable amount of time for view augmentation, we aim to make this process faster to fully leverage the advantages of single-test-image adaptation. In the future, it might involve end-to-end fine-tuning of the CLIP models, similar to Alpha-CLIP, using the principles proposed in this paper to obtain a model that can automatically overcome spurious features interference.

\section{Clarifications After Rebuttal}

We thank all reviewers for their suggestions. We organize the main clarifications during the rebuttal period as follows.

\question{Q: Why these specific works were chosen.}

We selected these methods because they belong to different types of approach and are representative.
There are two main approaches to adjust CLIP to against spurious features: region-aware methods and prompt tuning. Region-aware methods highlight the target by manipulating the image to make the model focus more on the desired object. Prompt tuning adapts the model to specific tasks by adjusting the prompts.
TPT is a representative prompt tuning method, while Alpha-CLIP is a representative region-aware method. Both methods have been proposed in the past two years and have demonstrated promising performance.

\question{Q: Discuss the previous works.}

These approaches differ from our method in terms of their setup, as they all utilize labeled training sets to identify and overcome spurious features through adaptation on the training set, whereas our approach focuses on adapting to individual test samples without relying on training sets or labels.

[a1]: firstly, accuracy dependence is estimated by comparing the presence/absence features to detect spurious correlations. Based on the identified spurious features, the Contrastive Loss train CLIP is designed to overcome decision shortcuts.

[a2]: the prompts foundation models to zero-shot predict the spurious attribute on a labeled dataset with spurious correlations, followed by finetuning the model based on the spurious attribute.

[a3]: the two projection layers are fine-tuned separately to fit the invariant image feature and the Spurious image feature in the labeled data, aiming to decouple the two types of feature.

Supervised methods generally outperform test-time adaptation. But in scenarios where accompanying labeled data is unavailable, these methods have limitations and would be impractical to deploy.

\question{Q: Computational cost.}

Compared to fine-tuning methods, our method that does not require fine-tuning has significantly lower computational cost.

The method proposed in this paper is on par with zero-shot methods in terms of cost.

\question{Q: Without spurious correlations.}

Test-time prompt optimization does not negatively impact performance on standard data without spurious correlations.

Our strategy is soft, so the method proposed in this paper does not adjust for cases where the background does not lead to decision shortcuts.
The experimental results also support this claim. There is a significant overall improvement in average performance in all categories.

\question{Q: Performance on CUB.}

As stated in our experimental setup, we present results on a subset consisting of the 10 most challenging classes (that is, 10 classes with the lowest accuracy in CLIP). This allows for a clear differentiation of the effectiveness of different methods.

Previous works [a4] [a5] report results on the entire dataset, which leads to performance differences of around 0.5\% (close to the variance) among different methods, making it difficult to intuitively reflect the differences between them.

\question{Q: Prompt-tuning methods like CoOp.}

CoOp generally outperforms our method because it involves supervised fine-tuning, whereas our approach focuses on adaptation for individual test samples without the need for training sets or labels.

Although methods like CoOp exhibit better performance, their application is limited in scenarios where accompanying labeled data are unavailable. Such methods would be impractical to implement.

\question{Q: The performance of the proposed method is significantly lower compared to [a6].}

The performance of the proposed method is noticeably inferior to that of [a6] because our approach involves on-the-fly test-time adaptation, whereas [a6] utilizes supervised contrastive optimization and performs correctness-based resampling, resulting in better performance.

\question{Q: WILDS benchmark.}

We did not report the results on WILDS because the decision shortcuts defined by it are not found in CLIP. The newly proposed benchmark is not more challenging than existing datasets, but rather includes the decision shortcuts present in CLIP.

The decision shortcuts in the WILDS dataset arise from carefully designed limited-scale training data, such as decision shortcuts between image style and label designed in the PACS dataset.

VLFMs (Vision-and-Language Fusion Models) are constructed using large-scale open-source data, which often leads to the absence of these designed decision shortcuts in VLFMs.

\textbf{If a model aims to demonstrate the designed decision shortcuts on the test set of WILDS, it needs to be trained on the training set of WILDS.}

Therefore, the WILDS benchmark is not suitable for evaluating the performance of foundation models.

References

[a1] \emph{Yang, Yu, et al. "Mitigating spurious correlations in multi-modal models during fine-tuning." ICLR 2023.}

[a2] \emph{Setlur, Amrith, et al. "Prompting for Robustness: Extracting Robust Classifiers from Foundation Models." ICLR 2024 Workshop on Reliable and Responsible Foundation Models.}

[a3] \emph{Zhang, Jie, et al. "Amend to Alignment: Decoupled Prompt Tuning for Mitigating Spurious Correlation in Vision-Language Models." ICML 2024.}

[a4] \emph{Visual classification via description from large language models, ICLR23}

[a5] \emph{Waffling around for Performance: Visual Classification with Random Words and Broad Concepts, ICCV23}

[a6]  \emph{Zhang and Ré, "Contrastive Adapters for Foundation Model Group Robustness." NeurIPS 2022.}
